# Supplementary material for: Thermodynamics-inspired Explanations of Artificial Intelligence
Source: arXiv:2206.13475 source file (2024-04-08)
Supplement: Supplementary file 1 [file SI.pdf]

# Supporting Information: Thermodynamics-inspired Explanations of Artificial Intelligence

**Shams Mehdi**[1] **and Pratyush Tiwary**[2,3,a]

[1]Biophysics Program and Institute for Physical Science and Technology, University of Maryland, College Park 20742, USA

[2]Department of Chemistry and Biochemistry and Institute for Physical Science and Technology, University of Maryland, College Park 20742, USA.

[3]University of Maryland Institute for Health Computing, Rockville, MD, USA.

[a] Electronic mail: ptiwary@umd.edu

## I. PROOFS

***Theorem 01:*** $\mathcal{S}_k$ is a monotonically increasing function of the number of features ($k$).

Let linear regression with $k$ features yields $k$ coefficients $(\{f_1, f_2, ..., f_k\}|1 < k \leq n)$. As discussed in the main text, we can define a probability distribution $p_k := \frac{|f_k|}{\sum_{i=1}^{n}|f_i|}$ and interpretation entropy ($\mathcal{S}_k$),

$$\mathcal{S}_k(p) = -\sum_{i=1}^{k} p_i \log p_i \quad (1)$$

Similarly, interpretation entropy for a $k+1$ coefficient model is given by,

$$\mathcal{S}_{k+1}(p') = -\sum_{i=1}^{k+1} p'_i \log p'_i \quad (2)$$

$\mathcal{S}_k$ is a monotonically increasing function iff,

$$\mathcal{S}_{k+1} - \mathcal{S}_k \geq 0 \quad (3)$$

Now, $\mathcal{S}_{k+1} = -\sum_{i=1}^{k} p'_i \log p'_i - p'_{k+1} \log p'_{k+1}$. If the features are independent, adding new features will not change the relative ratios of the existing features. *I.e,* $\frac{p_i}{p'_i} = \alpha$. In other words, we need to rescale the existing distribution by a single positive constant $\alpha$ to preserve the relative ratios, since $\sum_{i=1}^{k} p_i = \sum_{i=1}^{k+1} p'_i = 1$. Now,

$$\begin{aligned} \sum_{i=1}^{k+1} p'_i &= 1 \\ \sum_{i=1}^{k} p'_i + p'_{k+1} &= 1 \\ \sum_{i=1}^{k} \frac{p_i}{\alpha} + p'_{k+1} &= 1 \\ \frac{1}{\alpha} * 1 + p'_{k+1} &= 1 \\ p'_{k+1} &= 1 - \frac{1}{\alpha} \end{aligned} \quad (4)$$

Now,

$$\mathcal{S}_{k+1} = -\sum_{i=1}^{k} \frac{p_i}{\alpha} \log \frac{p_i}{\alpha} - p'_{k+1} \log p'_{k+1}$$

$$= -\sum_{i=1}^{k} \frac{p_i}{\alpha} \log p_i + \sum_{i=1}^{k} \frac{p_i}{\alpha} \log \alpha - (1 - \frac{1}{\alpha}) \log (1 - \frac{1}{\alpha}) \tag{5}$$

$$= +\frac{1}{\alpha}\mathcal{S}_k(p) + \frac{1}{\alpha} \log \alpha - (1 - \frac{1}{\alpha}) \log (1 - \frac{1}{\alpha})$$

$$\implies \mathcal{S}_{k+1}(p') - \mathcal{S}_k(p) = (\frac{1}{\alpha} - 1)\mathcal{S}_k(p) + \frac{1}{\alpha} \log \alpha - (1 - \frac{1}{\alpha}) \log (1 - \frac{1}{\alpha}) \tag{6}$$

The strategy here, is to rewrite the R.H.S of the above equation completely in terms of the parameter $\alpha$. Now, let's check the lower limit of $\alpha$. Since, the minimum of $p'_{k+1}$ is zero,

$$p'_{k+1} \geq 0$$
$$\frac{\alpha - 1}{\alpha} \geq 0 \tag{7}$$
$$\implies \alpha \geq 1$$

To check the upper limit of $\alpha$ we recognize that the probability ($p'_{k+1}$) of the newly added feature is less than or equal to the average of the existing probabilities.

$$p'_{k+1} \leq \frac{\sum_i p_i}{k}$$
$$p'_{k+1} \leq \frac{1}{k}$$
$$\frac{\alpha - 1}{\alpha} \leq \frac{1}{k} \tag{8}$$
$$\implies \alpha \leq \frac{k}{k-1} \implies k \leq \frac{\alpha}{\alpha - 1}$$

Now, the maximum value that the first term of R.H.S. of **Eq.** 6 can take is when the probability distribution ($p$) is uniform. Using Jensen's inequality, $\mathcal{S}_k(p) \leq \log k$. Thus,

$$\implies \mathcal{S}_{k+1}(p') - \mathcal{S}_k(p) \geq (\frac{1}{\alpha} - 1) \log k + \frac{1}{\alpha} \log \alpha - (1 - \frac{1}{\alpha}) \log (1 - \frac{1}{\alpha}) \tag{9}$$

Substituting the upper limit (**Eq.** 8) of $k$ in the above expression we get,

$$\mathcal{S}_{k+1}(p') - \mathcal{S}_k(p) \geq (\frac{1}{\alpha} - 1)\ \log\ \frac{\alpha}{\alpha - 1} + \frac{1}{\alpha}\ \log\ \alpha - (1 - \frac{1}{\alpha})\ \log\ (1 - \frac{1}{\alpha})$$
$$\implies \mathcal{S}_{k+1}(p') - \mathcal{S}_k(p) \geq \frac{1}{\alpha}\ \log\ \alpha \qquad (10)$$

Since, $\alpha$ is a positive constant, this shows that $\mathcal{S}_k$ increases monotonically with $k$, if the features are independent. When the rescaling factor $\alpha = 1$ *i.e,* when no additional feature is added the R.H.S. of the above expression becomes zero.

***Theorem 02:*** $\mathcal{S}$ monotonically increases as $\mathcal{U}$ decreases.

Since, the linear regressions are performed with standardized data, if the probability ($p_i$) of a feature is relatively high, the feature is understood to have a high contribution towards predictions. However, a high probability value makes the distribution less sharply peaked *i.e,* high $\mathcal{S}$ compared to a low probability value. Thus, in practice $\mathcal{S}$ monotonically increases as $\mathcal{U}$ decreases.

An illustrative $\mathcal{U}$ vs. $\mathcal{S}$ profile is shown in **Fig.** 1.

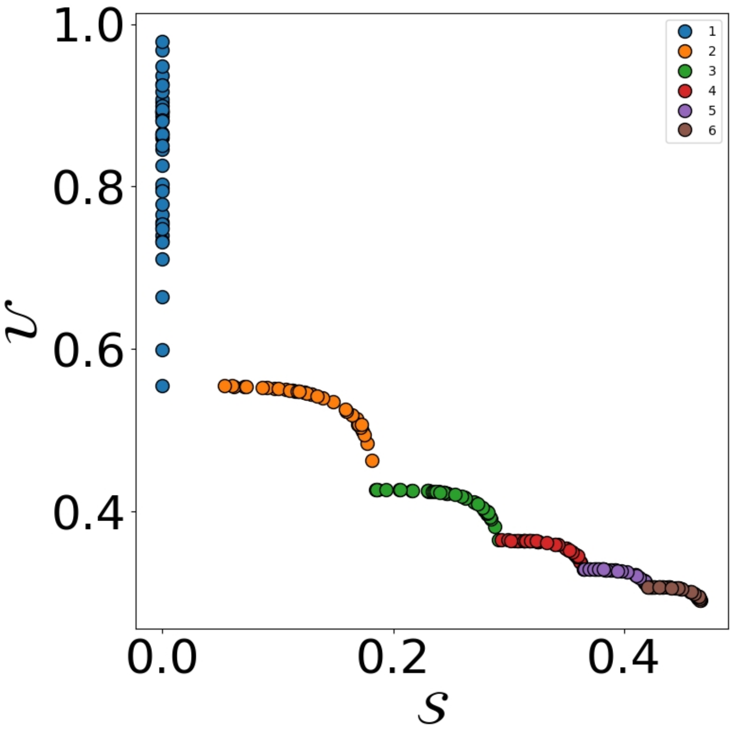


**Supporting Figure 1:** Illustrative $\mathcal{U}$ vs. $\mathcal{S}$ plot. The different colors correspond to the linear regression of $k = 1, 2, 3, 4, 5, 6$ coefficient models respectively.

***Lemma 02:*** Existence of a global minimum.

The exact values of unfaithfulness $\mathcal{U}$, and interpretation entropy $\mathcal{S}$ functions depend on the nature of the problem/data. For practical problems, $\mathcal{U}$ plateaus with high $k$ *i.e,* $\frac{\Delta \mathcal{U}}{\Delta k} \approx 0$, while $\mathcal{S}$ has a lower limit of $\frac{1}{\alpha} \log \alpha$ as shown in **Theorem 01**. As a result, when $\theta$ is increased slowly from zero, $\frac{\Delta \mathcal{S}}{\Delta k}$ dominates $\frac{\Delta \mathcal{U}}{\Delta k}$ at high $k$, while at low $k$ $\frac{\Delta \mathcal{U}}{\Delta k}$ dominates $\frac{\Delta \mathcal{S}}{\Delta k}$. This phenomenon produces the desired global minima at the optimal $k$ coefficient model at a specific temperature $\theta$.

## II. STRATEGY FOR ANALYZING HIGH NUMBER OF FEATURES

TERP implements a forward feature selection through linear regression, and the number of analyzed models can increase greatly with the number of features. A simple strategy to address this is the implementation of a pre-processing round of linear regression to identify and discard near-zero coefficient features prior to implementing TERP.

## III. APPLICATION TO AI-AUGMENTED MD: VAMPNETS

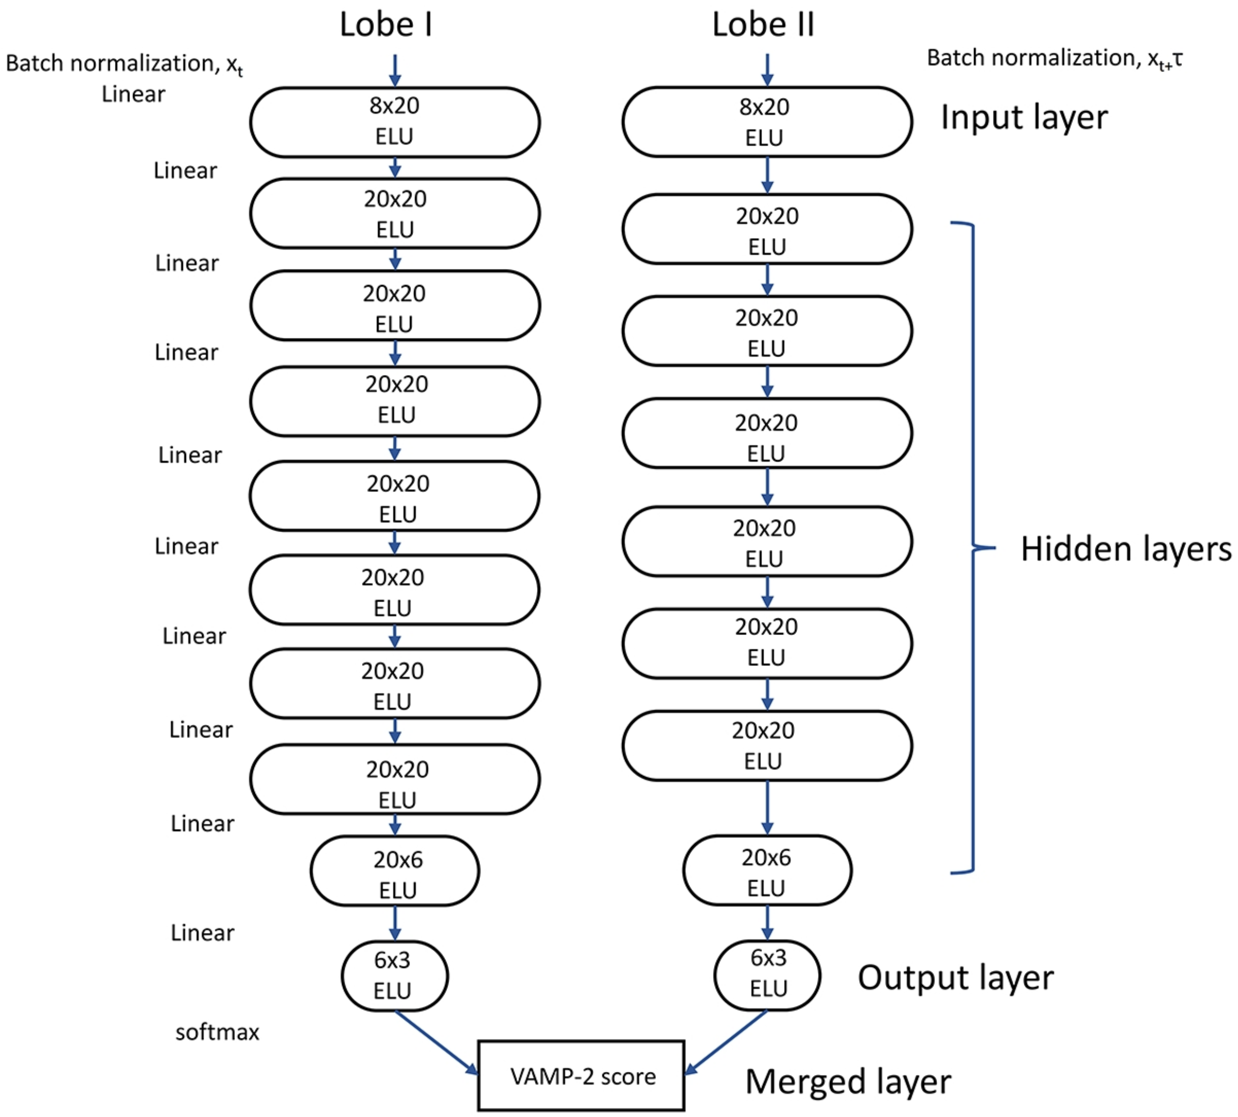


**Supporting Figure 2:** VAMPnets architecture.

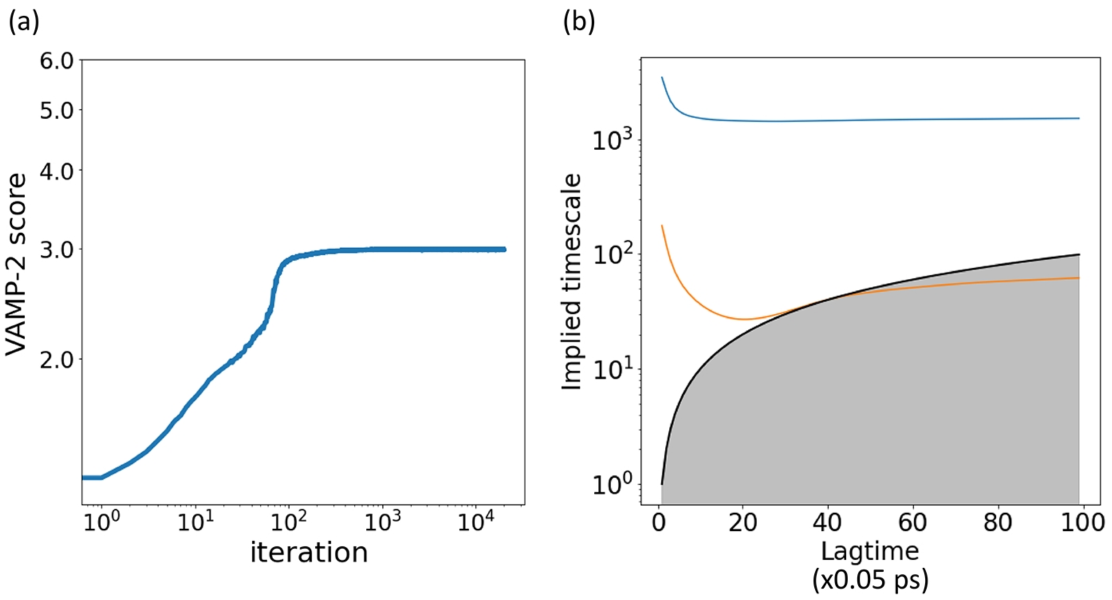


**Supporting Figure 3:** (a) Maximized VAMP-2 score for 50 training epochs, (b) Implied timescale vs. lagtime $\tau$ for second and third eigenvectors represented by blue and orange colors corresponding to transitions between different metastable states. Timescales within the grey region are faster than $\tau$ and cannot be resolved by the VAMPnets model.[1]

## IV. APPLICATION TO IMAGE CLASSIFICATION: VISION TRANSFORMERS (VITS)

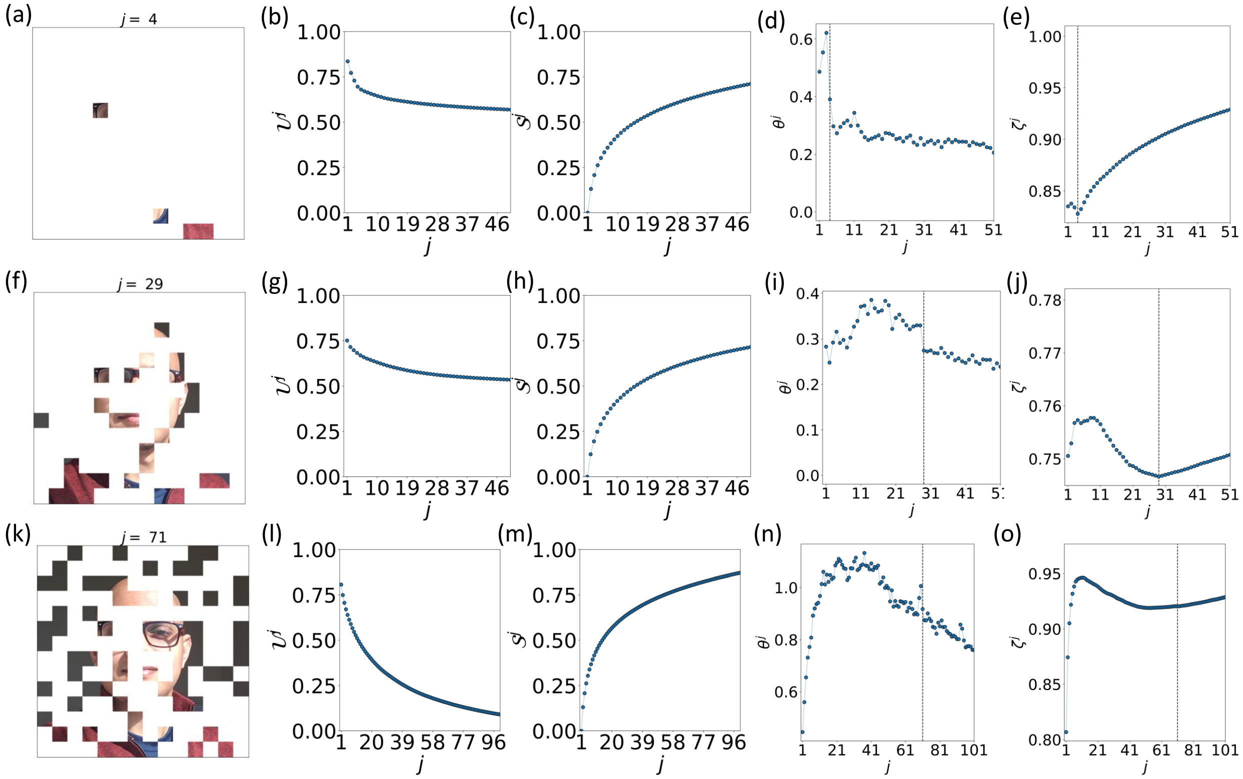


**Supporting Figure 4:** TERP results for parameter and data randomization sanity checks. For ViT prediction 'Eyeglasses', panels (a-e) show TERP optimal explanation, $\mathcal{U}^j$, $\mathcal{S}^j$, $\theta^{|}$, and $\zeta^j$ when all the parameters in ViT architecture blocks $11-6$ were randomized i.e, drawn from a normal distribution. Panels (f-j) show results when all the parameters in ViT architecture blocks $11-3$ were randomized. Panels (k-o) show results for the data randomization test i.e, when a new ViT model is trained by randomizing all the labels associated with each sample in the training set during training.

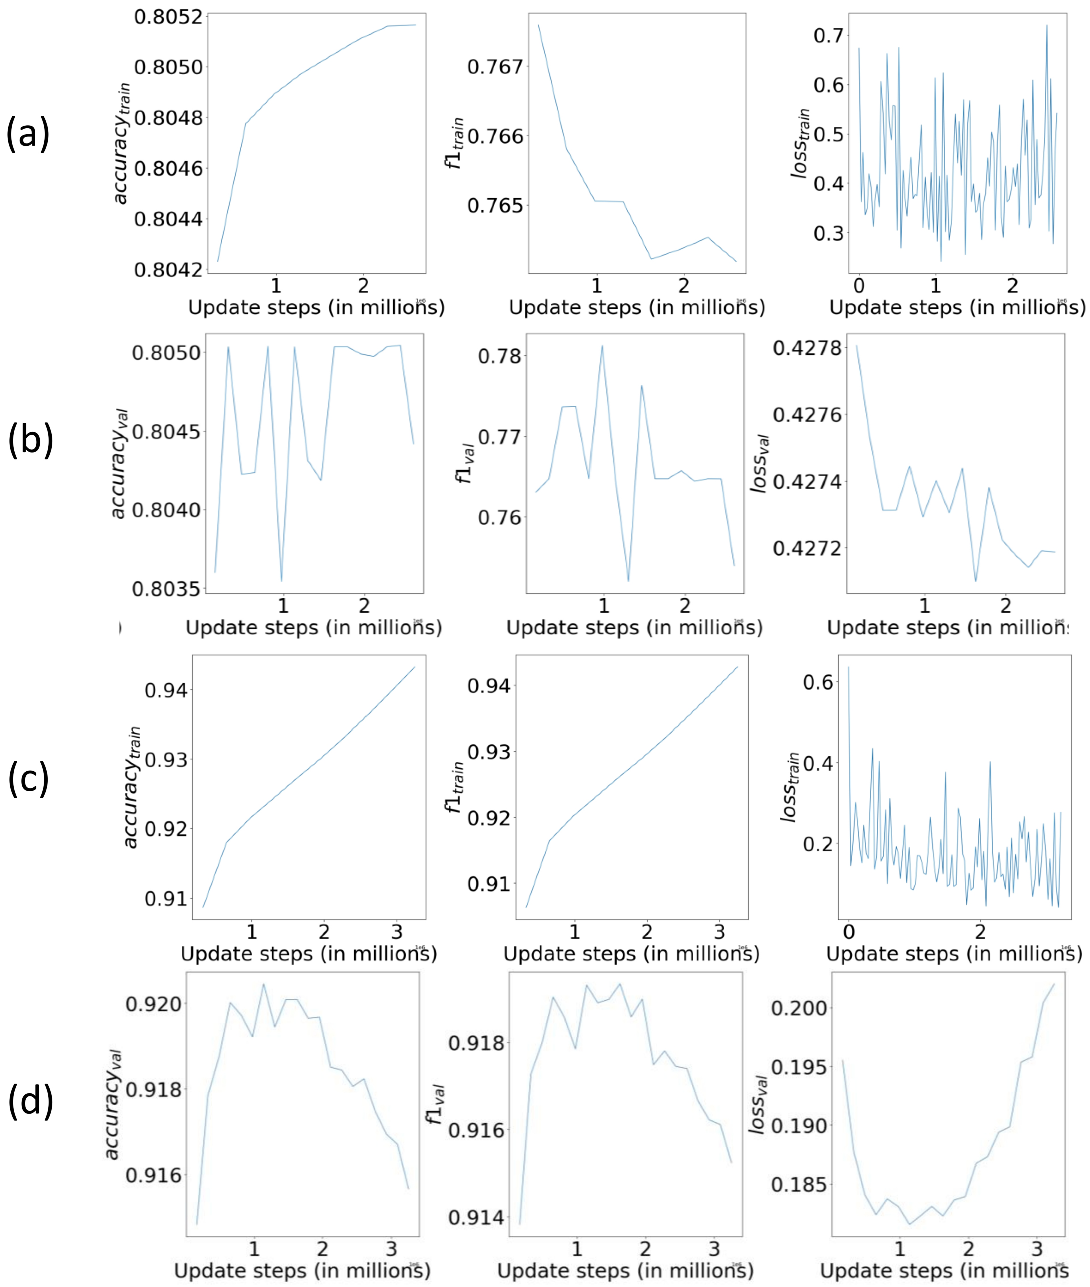


**Supporting Figure 5:** ViT model performance metrics (accuracy, f1 score, and binary cross entropy loss) as a function of model parameter updates. (a) Training, (b) validation of the fine-tuned model. (c) Training, (d) validation of the data randomized model. All the models were trained using a batch size of 1. Thus, during training, parameters were updated each time an image was passed to the model.

## References

[1] A. Mardt, L. Pasquali, H. Wu, and F. Noé, Nature communications **9**, 1 (2018).
